# Supplementary material for: GPT-4V as Traffic Assistant: An In-depth Look at Vision Language Model on Complex Traffic Events
Source: arXiv:2402.02205 source file (2024-02-07)
Supplement: Supplementary file 1 [file 6_Appendix.tex]

\appendices
\section{What Goes in the Appendices} \label{App:WhatGoes}
The appendix is for material that readers only need to know if they are studying the report in depth. Relevant charts, big tables of data, large maps, graphs, etc. that were part of the research, but would distract the flow of the report should be given in the Appendices. 
\section{Formatting the Appendices} \label{App:Formatting}
Each appendix needs to be given a letter (A, B, C, etc.) and a title. \LaTeX will do the lettering automatically.
